# Supplementary material for: Misinformation as a harm: structured approaches for fact-checking prioritization
Source: arXiv:2312.11678 source file (2024-03-18)
Supplement: Supplementary file 1 [file AppendixA-redacted.pdf]

# Urgent Questions

## A Structured Response to Misinformation as Harm

In fact checking, a critical need is prioritization. Focusing on the challenge of misinformation, how can fact checkers be supported in their decision making to decide which pieces of content may have more negative impacts in comparison to others? Five major dimensions can help determine the potential urgency of a specific message or post: **actionability**, **exploitativeness**, **likelihood of spread**, **believability**, and **social fragmentation**. A longer version of the questionnaire with helpful hints for answering can be found at:

### Urgency Dimension 1: Actionability

A piece of content is more harmful the more that it spurs actions that directly cause harm. Therefore, a piece of misinformation is more harmful the more that it spurs direct action.

Mark a "1" for each answer and tally them up.

Suggestions for hints on how to answer these questions can be found at

Use the Key Questions if a quick assessment is needed highlighted in (dark blue).

"Don't Know/Not Applicable" (?) can be subtracted from Total "Yes" (Y) answers to gain a relative magnitude of urgency across different pieces of content.

| Actionability Questions                                                                                                                                                                                                               | Y | N | ? |
|---------------------------------------------------------------------------------------------------------------------------------------------------------------------------------------------------------------------------------------|---|---|---|
| Does the message content include an explicit call to action?                                                                                                                                                                          |   |   |   |
| Does the piece of content incorporate coordination efforts, such as dates/times or other arrangements for follow-up?                                                                                                                  |   |   |   |
| Does the message provide a name or otherwise any identifying information about an individual, an address, or a place of work in such a way that people might be directly harmed?                                                      |   |   |   |
| Does the message content include a tone of urgency or mention of time sensitivity?                                                                                                                                                    |   |   |   |
| Does the message content include any threats of violence?                                                                                                                                                                             |   |   |   |
| Does the message lay blame or cast aspersions or hatred on a particular group, such as a particular religion, gender, sexual orientation, race, country, or culture, that has been harmed in the past by the audience of the content? |   |   |   |
| Does the message invoke a sense of injustice or moral outrage, including on behalf of a vulnerable individual or group such as children or women?                                                                                     |   |   |   |
| Does the direct target or current audience members directly addressed of the message have a recent history of taking actions that cause harm?                                                                                         |   |   |   |
| Is this message associated with/similar to other messages that are also actionable?                                                                                                                                                   |   |   |   |
| Subtotal:                                                                                                                                                                                                                             |   |   |   |

## Urgency Dimension 2: Exploitativeness

A piece of misinformation is more harmful the more the message seeks to exploit human or a group's weaknesses, including a lack of resources.

Mark a "1" for each answer and tally them up.

Suggestions for hints on how to answer these questions can be found at

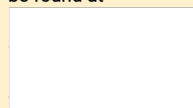

Use the Key Questions if a quick assessment is needed highlighted in (dark blue).

*"Don't Know/Not Applicable" (?) can be subtracted from Total "Yes" (Y) answers to gain a relative magnitude of urgency across different pieces of content.*

| Exploitativeness Questions                                                                                                                                            | Y | N | ? |
|-----------------------------------------------------------------------------------------------------------------------------------------------------------------------|---|---|---|
| Does the message directly address or reference children or use language aimed at a younger audience?                                                                  |   |   |   |
| Does the message directly address or reference elderly community members, or discuss topics aimed at them?                                                            |   |   |   |
| Does the message introduce a degree of fear or feelings of uneasiness?                                                                                                |   |   |   |
| Is the message content complicated to understand?                                                                                                                     |   |   |   |
| Does the message directly address or reference military veterans, or discuss topics aimed at them?                                                                    |   |   |   |
| Does the message make mention of a reader's feelings of isolation?                                                                                                    |   |   |   |
| Does the message make mention of a reader's feelings of powerlessness?                                                                                                |   |   |   |
| Does the message make mention of a reader's feelings of disenfranchisement?                                                                                           |   |   |   |
| Is this message associated with/similar to other messages that are also actionable?                                                                                   |   |   |   |
| Is the language of the intended audience neither a UN language (English, French, Spanish, Mandarin Chinese, Russian) nor on the top 5 list of most popular languages? |   |   |   |
| Is the message presented in a region where the local context might amplify its harm?                                                                                  |   |   |   |
| <b>Subtotal:</b>                                                                                                                                                      |   |   |   |

### Urgency Dimension 3a: Likelihood of Spread

A piece of harmful content is more harmful the more places it appears, and the more people are exposed to it. Therefore, a piece of misinformation is more harmful the more places and people are exposed to it.

Mark a "1" for each answer and tally them up. Suggestions for hints on how to answer these questions can be found at

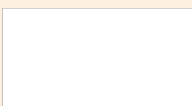

Use the Key Questions if a quick assessment is needed highlighted in (dark blue).

| Likelihood of Spread Questions |                                                                                                                                                                            | Y | N | ? |
|--------------------------------|----------------------------------------------------------------------------------------------------------------------------------------------------------------------------|---|---|---|
| WHO is spreading?              | Is the content already spreading far and/or fast on a multitude of platforms?                                                                                              |   |   |   |
|                                | Do the people or entities who are spreading the piece of content have a broad reach (size of following on social media, "influencer," presence on TV or other news media)? |   |   |   |
|                                | Are the people or entities known to be repeat spreaders of questionable information?                                                                                       |   |   |   |
| WHERE is it spreading?         | Is there evidence of coordination activity (whether bot/automated or not) to encourage spread?                                                                             |   |   |   |
|                                | Is the content publicly accessible (posted on a public platform, addressable URL)? Is the content posted on a popular platform?                                            |   |   |   |
|                                | Is the content spreading on multiple platforms?                                                                                                                            |   |   |   |
|                                | Does one of the platforms upon which the content is shared have tools to support amplification (e.g. reshares, algorithmic feeds, recommendation engines)?                 |   |   |   |

...Urgency Dimension questions continue on next page

"Don't Know/Not Applicable" (?) can be subtracted from Total "Yes" (Y) answers to gain a relative magnitude of urgency across different pieces of content.

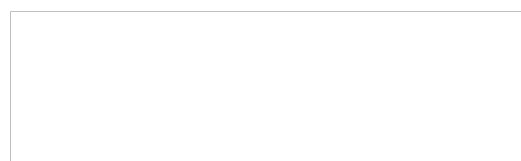

**Urgency  
Dimension 3b:  
Likelihood of  
Spread**

A piece of harmful content is more harmful the more places it appears, and the people are exposed to it. Therefore, a piece of misinformation is more harmful the more places and people are exposed to it.

**Mark a "1" for each answer and tally them up.**  
Suggestions for hints on how to answer these questions can be found at

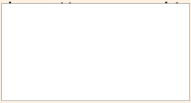

Use the Key Questions if a quick assessment is needed highlighted in (dark blue).

*"Don't Know/Not Applicable" (?) can be subtracted from Total "Yes" (Y) answers to gain a relative magnitude of urgency across different pieces of content.*

| Likelihood of Spread Questions |                                                                                                                                                                 | Y | N | ? |
|--------------------------------|-----------------------------------------------------------------------------------------------------------------------------------------------------------------|---|---|---|
| CHARACTERISTICS of the message | Does the message make direct appeals to audience members that it in their financial, political, or social interest to spread the content further?               |   |   |   |
|                                | Does the message directly call audience members to share the content further?                                                                                   |   |   |   |
|                                | Is the tone of the content striking enough in ways that encourage sharing?                                                                                      |   |   |   |
|                                | Does the content contain an image, audio-clip, or other richer formats that are easy to remember, visually or aurally arresting, or seems interesting to share? |   |   |   |
|                                | Does the message impart a sense of exclusivity or novelty ("breaking news")?                                                                                    |   |   |   |
|                                | Are there hashtags associated with the message?                                                                                                                 |   |   |   |
|                                | Is the message difficult to fact-check or prove false?                                                                                                          |   |   |   |
|                                | Is the message related to a current event or a topic that is being reported on actively by many news outlets ?                                                  |   |   |   |
|                                | <b>Subtotal:</b>                                                                                                                                                |   |   |   |

**Instructions:**

Please tally 3a and 3b totals in Subtotal, above right.

### Urgency Dimension 4: Believability

A piece of misinformation is more harmful the more believable its message is to a specific community.

Mark a "1" for each answer and tally them up.

Suggestions for hints on how to answer these questions can be found at

Use the Key Questions if a quick assessment is needed highlighted in (dark blue).

"Don't Know/Not Applicable" (?) can be subtracted from Total "Yes" (Y) answers to gain a relative magnitude of urgency across different pieces of content.

| Believability Questions                                                                                                                                          | Y | N | ? |
|------------------------------------------------------------------------------------------------------------------------------------------------------------------|---|---|---|
| Is there a lack of high quality information that is publicly accessible and is refuting the message's claim?                                                     |   |   |   |
| Does the poster and/or organization/outlet have a noteworthy number of social media/community followers?                                                         |   |   |   |
| Is the content published by an organization/outlet with uncertain editorial control (e.g. is not a recognized news publisher)?                                   |   |   |   |
| Does the message fail to include external citations, links, or language about evidence to support its claim?                                                     |   |   |   |
| Does the message contain richer formats as part of its evidence that lay people consider to have low falsifiability?                                             |   |   |   |
| Is the message written or communicated in a personal or persuasive tone?                                                                                         |   |   |   |
| Does the message make reference to the broad believability of the claim or topic?                                                                                |   |   |   |
| Does the message appeal to a specific community identity by mentioning a shared set of values or beliefs?                                                        |   |   |   |
| Is there a lack of consensus on the part of experts regarding the claim?                                                                                         |   |   |   |
| Does the poster have credentials that represents some kind of expertise?                                                                                         |   |   |   |
| Is the content posted by an imposter individual or counterfeit outlet that could successfully pass as a different person/account based only upon a quick glance? |   |   |   |
| Does the content have the graphics and styling of a legitimate news agency or mainstream information source?                                                     |   |   |   |
| Subtotal                                                                                                                                                         |   |   |   |

## Urgency Dimension 5: Social Fragmentation

A piece of misinformation could have indirect, societal, and accumulative effects. Therefore, a piece of misinformation is potentially more harmful the more that it addresses or is part of societal and community relationships over time.

There are no short cut questions for this category.

Mark a "1" for each answer and tally them up.

Suggestions for hints on how to answer these questions can be found at

Use the Key Questions if a quick assessment is needed highlighted in (dark blue).

| Social Fragmentation Questions                                                                            | Y | N | ? |
|-----------------------------------------------------------------------------------------------------------|---|---|---|
| Does the message fit into a larger narrative that has been existing for some time?                        |   |   |   |
| Does the message question trust in or the functioning of public institutions?                             |   |   |   |
| Does the message question trust in or the functioning of the scientific community as a whole?             |   |   |   |
| Does the message question the functioning of or trust in news sources/ the media in general?              |   |   |   |
| Does the message question the trustworthiness of other people in general within a community or society?   |   |   |   |
| In a democratic country where there are elections, does the message directly attack the election process? |   |   |   |
| Subtotal                                                                                                  |   |   |   |

| Urgency<br>Dimension 1:<br>Actionability | Urgency<br>Dimension 2:<br>Exploitativeness | Urgency<br>Dimension 3:<br>Likelihood of<br>Spread | Urgency<br>Dimension 4:<br>Believability | Urgency<br>Dimension 5:<br>Social<br>Fragmentation | TOTAL |
|------------------------------------------|---------------------------------------------|----------------------------------------------------|------------------------------------------|----------------------------------------------------|-------|
|                                          |                                             |                                                    |                                          |                                                    |       |

"Don't Know/Not Applicable" (?) can be subtracted from Total "Yes" (Y) answers to gain a relative magnitude of urgency across different pieces of content.
